# Supplementary material for: Estimating Social Network Models with Link Misclassification
Source: arXiv:2509.07343 source file (2026-10-30)
Supplement: Supplementary file 1 [file appendix_to_arXiv_202509.tex]

\documentclass[final,12pt]{article}
%%%%%%%%%%%%%%%%%%%%%%%%%%%%%%%%%%%%%%%%%%%%%%%%%%%%%%%%%%%%%%%%%%%%%%%%%%%%%%%%%%%%%%%%%%%%%%%%%%%%%%%%%%%%%%%%%%%%%%%%%%%%%%%%%%%%%%%%%%%%%%%%%%%%%%%%%%%%%%%%%%%%%%%%%%%%%%%%%%%%%%%%%%%%%%%%%%%%%%%%%%%%%%%%%%%%%%%%%%%%%%%%%%%%%%%%%%%%%%%%%%%%%%%%%%%%
\usepackage{amssymb}
\usepackage{amsfonts}
\usepackage{amsmath}
\usepackage{geometry}
\usepackage{amsthm}
\usepackage{hyperref,backref}
\usepackage[comma]{natbib}
\setlength{\bibsep}{6pt}
\usepackage{xcolor}
\usepackage{graphicx}
\usepackage{setspace}
\usepackage[bottom]{footmisc}
\usepackage{scalefnt}
\newcounter{aprop} % Define a custom counter
 % Define how the number will appear (e.g., A1, A2, ...)
\newtheorem{aproposition}[aprop]{Proposition} % Define the new theorem environment using that counter

\setcounter{MaxMatrixCols}{10}

\geometry{top=1.1in,bottom=1.05in,right=1.05in,left=1.05in}

\begin{document}
\begin{spacing}{1.5}

\title{Online Appendix: Estimating Social Network Models with Link Misclassification}
\author{Arthur Lewbel, Xi Qu, and Xun Tang}
\date{%
%TCIMACRO{\TeXButton{Current Date}{\today}}%
%BeginExpansion
\today%
%EndExpansion
}
\maketitle

% \section{A Single Large Network} \label{sec:single_large}
\section{Extensions of the Benchmark Model} \label{sec:extension}

We now extend the method in Section 3 in the main text to more general settings with contextual effects, heterogeneous misclassification rates, or group fixed effects. 
We focus on extending the ideas for constructive identification. 
Estimation in each case follows from an analog principle and similar steps as in Section 4. To simplify exposition, we let group sizes $n_s =n$ be fixed throughout the remainder of this section. 

\subsection{Contextual effects}

Suppose the structural form, based on perfect observation of the actual adjacency $G$, is:
\begin{equation*}
y=\lambda Gy+X\beta +GX\gamma +\varepsilon \text{,}
\end{equation*}%
where $\gamma $ are contextual effects showing how individual outcomes are directly influenced by the characteristics of others linked to the individual.
The feasible structural form, based on $H$ and subject to misclassification errors, is: $y=\lambda Wy + X\beta + WX \gamma +\eta$, 
where $W\equiv [H-p_0(\iota\iota' -I)]/(1-p_0-p_1)$ as before, and the composite error $\eta$ is: $\eta \equiv \varepsilon -\lambda \left( W-G\right) y-\left( 
W-G\right) X\gamma$.

Under the same conditions and by the same arguments as in the case with no contextual effects in Section 3, we can show that the new composite error $\eta $ is mean-independent from $(X,G)$.
Similarly, we can construct instruments using network measures $H$ as before. 
Our next proposition establishes these results. 
For generality, let $\zeta(X)\in \mathbb{R}^{n\times L}$ be any generic function of $X$ with $L\geq K$.

\begin{aproposition}
\label{pn:HX_context} Suppose (A1), (A2), and (A3) hold. Then $E(\eta|X,G)=0 $. If in addition (A4) holds, then $E [\zeta \left(X\right)^{\prime }W\eta] = E[\zeta\left(X\right)^{\prime}H\eta] = 0$.
\end{aproposition}

\begin{proof}[Proof of Proposition \protect\ref{pn:HX_context}]
Under (A3),
\begin{eqnarray*}
E(Gy|X,G) &=&E[GM(X\beta +GX\gamma +\varepsilon )|X,G]=GM\left( X\beta
+GX\gamma \right) \text{,} \\
E(Wy|X,G) &=&E[WME\left( X\beta +GX\gamma +\varepsilon |X,G,H\right)
|X,G]=E(W|G,X)M(X\beta +GX\gamma )\text{.}
\end{eqnarray*}%
Under (A1) and (A2), $E(W|G,X)=G$. It then follows that $E(\eta |X,G)=0$. 

Next, note 
\begin{eqnarray*}
E\left[ \zeta (X)^{\prime }W Wy|G,X\right]  &=&\zeta \left( X\right) ^{\prime
}E(W^{2}|G,X)M(X\beta +GX\gamma )\text{; } \\
E[\zeta \left( X\right) ^{\prime }W WX|G,X] &=&\zeta \left( X\right) ^{\prime
}E(W^{2}|G,X)X\text{; } \\
E\left[ \zeta (X)^{\prime }WGy|G,X\right]  &=&\zeta \left( X\right) ^{\prime
}E(W|G,X)GM(X\beta +GX\gamma )\text{; } \\
E[\zeta \left( X\right) ^{\prime }WGX|G,X] &=&\zeta \left( X\right) ^{\prime
}E(W|G,X)GX\text{.}
\end{eqnarray*}%
As shown in the appendix of the main text, under (A4), $E(W^{2}|G,X)=G^2$. 
Because $E(W|G,X)=G$ under (A1) and (A2), this implies $E\left[ \zeta \left( X\right) ^{\prime }W\eta \right] =0$.
Also, $ E[\zeta(X)'H\eta] = (1-p_0-p_1) E[\zeta(X)'W\eta] + E[\zeta(X)'p_0(\iota\iota'-I)\eta] = 0$, where the second equality holds because $E(\eta|X,G)=0$.
\end{proof}

This proposition implies that $H^{\prime }\zeta (X)$ and $W^{\prime} \zeta(X)$ satisfy instrument exogeneity for generic functions of $X$. 
In fact, a stronger result holds under (A1)-(A4): $E(W \eta|G,X)=E(H\eta |G,X)=0$. 
The intuition is the same as in Proposition 2. 
Thus we can apply 2SLS as before to consistently estimate $(\lambda,\beta ^{\prime },\gamma ^{\prime })^{\prime }$ using $(H^{\prime}X,X,H^{\prime }\zeta (X))$ as instruments for $\left( Wy,X,WX\right) $, provided the appropriate rank conditions hold.

\subsection{Heterogeneous misclassification rates}

We now allow the misclassification rates $p_{0},p_{1}$ to vary with individual characteristics $X$. To fix ideas, we return to the case with no contextual effects as in Section 3. 
Generalization to include contextual effects, using the results from the preceding sub-section, is immediate.

Suppose we relax Assumption (A2) as follows:%
\begin{equation*}
\text{(A2') }E(H_{ij}|G_{ij}=1,X)=1-p_{ij,1}(X)\text{ and }%
E(H_{ij}|G_{ij}=0,X)=p_{ij,0}(X)\text{ }\forall i\not=j\text{.}
\end{equation*}%
Define 
\begin{equation*}
W_{ij}(X)\mathcal{\equiv }\frac{H_{ij}-p_{ij,0}(X)}{%
1-p_{ij,0}(X)-p_{ij,1}(X)}\text{ if }i\not=j\text{, and }W%
_{ii}(X)=0\text{.}
\end{equation*}%
Under (A2'), $E[W_{ij}(X)|G,X]=1$ for $G_{ij}=1$, and $E[W_{ij}(X)|G,X]=0$ for $G_{ij}=0$. 
Hence $E(W(X)|G,X)=G$.

To recover misclassification rates $p_{ij,1}(\cdot )$ and $p_{ij,0}(\cdot )$, we can apply methods in Section 3.4 to pairwise links $G_{ij}$ and conditioning on $X$. 
In practice, we can mitigate the curse of dimensionality by specifying the rates $p_{ij,1}(X)$ and $p_{ij,0}(X)$ as functions of $X_{i}$ and $X_{j}$.

With knowledge of these heterogeneous misclassification rates, we can use adjusted 2SLS to consistently estimate $(\lambda ,\beta ^{\prime })^{\prime} $ from a feasible structural form:
\begin{equation*}
y=\lambda W(X)y+X\beta +\underset{v^{\ast }}{\underbrace{%
\varepsilon +\lambda \lbrack G-W(X)]y}}\text{.}
\end{equation*}%
Under (A2') and (A3),%
\begin{eqnarray}
&&E(v^{\ast }|G,X)=\lambda \{GE(y|G,X)-E\left[ \left. W%
(X)y\right\vert G,X\right] \}  \notag \\
&=&\lambda \{GMX\beta -E\left[ W(X)|G,X\right] MX\beta \}=\lambda
(G-G)MX\beta =0\text{.}  \label{EXO2}
\end{eqnarray}

\noindent Let $R^{\ast }\equiv \left( W(X)y,X\right) $ and $Z^{\ast }\equiv
(\zeta (X),X)$ where $\zeta (X)\in \mathbb{R}^{n\times L}$ is a nonlinear
function of $X$ with $L\geq K$ (e.g., $\zeta (X)\equiv X\circ X$, where $\circ$ denotes the Hadamard product of matrices). Then (\ref%
{EXO2}) implies $E(Z^{\ast \prime }v^{\ast })=0$. If $E(R^{\ast \prime
}Z^{\ast })$ and $E(Z^{\ast \prime }Z^{\ast })$ have full rank, we can use
this adjusted 2SLS to consistently estimate $(\lambda,\beta')'$.%

\subsection{Group fixed effects}

Suppose there is group-level unobserved heterogeneity $\alpha $ in the DGP: $y=\lambda Gy+X\beta +\alpha +\varepsilon $. We can implement the \textquotedblleft with-in\textquotedblright\ transformation on the adjusted network measure $W$, as in fixed-effect estimation of linear panel data models, to get $\mathcal{\dot{W}\equiv }\left[ I-\iota \iota'/n \right] W$. Essentially, this transformation just corresponds to demeaning $W$ within groups. Similarly, define with-in transformations on $y,\varepsilon ,X,G$ to obtain $\dot{y},\dot{\varepsilon},\dot{X},\dot{G}$ respectively. 
The resulting demeaned version of the structural form is:
\begin{equation}
\dot{y}=\lambda \mathcal{\dot{W}}y+\dot{X}\beta +\underset{\equiv \dot{v}}{%
\underbrace{\dot{\varepsilon}+\lambda(\dot{G}-\mathcal{\dot{W})}y}}. 
\end{equation}
Because $\dot{G}$ and $\mathcal{\dot{W}}$ are linear functions of $G$ and $H$ respectively, the same argument as Lemma 1 in Section 3 applies to show that $E(\dot{v}|X,G)=E(\dot{v}|\dot{X},\dot{G})=0$. 
Note that the presence of group fixed effects does not affect our method for recovering the misclassification rates in Section 3.4. 
With multiple network measures $H^{(t)}$ for $t=1,2$, we can apply adjusted 2SLS as in Section 4 to estimate $(\lambda ,\beta ^{\prime})^{\prime }$, using $\dot H^{(2)}X$ as instruments for $\mathcal{\dot{W}}^{(1)}y$.

\section{General Formula for $\mathbf P_{(H^*_{i\cdot}| G^*_{i\cdot})}$ in Section 3.6} % 

Define a 2-by-2 matrix $T \equiv [1-p_0 \text{ , } p_0 \text{ ; } p_1 \text{ , }1-p_1]$. 
Let $\mathcal G_n$ be a $2^{n-1}\times (n-1)$ matrix whose rows enumerate the joint support of $n-1$ binary variables.
That is, $\mathcal G_n$ is the support of $(G^*_{ij})_{j\neq i}$, and by construct also that of $(H^*_{ij})_{j\neq i}$, in a group with $n$ members.
Specifically, 
\begin{equation*}
\mathcal G_3 = \left( 
\begin{array}{cc}
0 & 0 \\ 0 & 1 \\ 1 & 0 \\ 1 & 1%
\end{array}%
\right) \text{ ; and }
\mathcal G_{n+1}=\left( 
\begin{array}{cc}
0_{2^{n-1}\times 1} & \mathcal G_n \\ 
1_{2^{n-1}\times 1} & \mathcal G_n %
\end{array}%
\right) \text{ for } n\geq 3.
\end{equation*}

For a group with $n$ members, let $\mathbf P_{(H^*_{i\cdot}\vert G^*_{i\cdot})}$ be the $2^{n-1}$-by-$2^{n-1}$ matrix of conditional probability of $ H^*_{i\cdot} $ given $ G^*_{i\cdot} $. 
The rows and columns of this matrix are labeled by the realizations of the vector of off-diagonal components $(G^*_{ij})_{j\neq i}$ and $(H^*_{ij})_{j\neq i}$ respectively. 
In particular, these row and column labels are aligned in the same order as the rows in $\mathcal G_n$ defined above.

Proposition 4 states that the general formula for the probability mass of $ H^*_{i\cdot} $ given $ G^*_{i\cdot} $, for a group with size $n$, is: 
\begin{eqnarray*}
\mathbf{P}_{(H_{i.}^{\ast }|G_{i.}^{\ast })} &=& T^{\otimes (n-1)} \equiv \underset{%
n-1}{\underbrace{T\otimes T\otimes \cdots \otimes T}}.
\end{eqnarray*}
It is thus convenient to calculate the inverse as 
\( (T^{\otimes (n-1)})^{-1} = \underset{n-1}{\underbrace{T^{-1}\otimes T^{-1}\otimes \cdots \otimes T^{-1}}}\).

We prove Proposition 4 by induction. 
First, for $n=3$, it is straightforward to verify that the conditional probability mass in Example 1 conforms to the formula $T^{\otimes 2} \equiv T\otimes T$. 
Next, suppose for a group with $n\geq 3$, the probability mass of $(H^*_{ij})_{j\neq i}$ conditional on $(G^*_{ij})_{j\neq i}$ is given by $T^{\otimes (n-1)}$.
% Recall how we define and order the rows in $\mathcal G_n$ for $n\geq 3$. 
Expand $(H^*_{ij})_{j\neq i}$ and $(G^*_{ij})_{j\neq i}$ by inserting an additional binary component in each, i.e., let the group size grow to $n+1$. 
Given how we define and order the rows in $\mathcal G_n$ for $n\geq 3$, the conditional probability mass for the expanded group with $n+1$ members, according to the right-hand side of the formula 
\begin{equation*} \label{eq:CPM}
    P(H^*_{i\cdot}\vert G^*_{i\cdot}) = \prod_{j\neq i} \left[(1-p_1)^{H^*_{ij}G^*_{ij}}(p_1)^{(1-H^*_{ij})G^*_{ij}}(p_0)^{H^*_{ij}(1-G^*_{ij})}(1-p_0)^{(1-H^*_{ij})(1-G^*_{ij})}\right],
\end{equation*}is
\begin{equation*}
\left( 
\begin{array}{cc}
(1-p_0)T^{\otimes (n-1)} & p_0 T^{\otimes (n-1)} \\ 
p_1 T^{\otimes (n-1)}& (1-p_1)T^{\otimes (n-1)}%
\end{array}%
\right) \equiv T^{\otimes n}.
\end{equation*}
% This proves the general formula in Proposition \ref{pn:generalCPM}.

\section{Asymptotics of the Adjusted 2SLS Estimator}

We derive the limiting distribution of our adjusted 2SLS estimator for the structural effects $\hat{\lambda}$ and $\hat{\beta}$ in Proposition 5 of Section 4. 

Recall from Section 4 that we have defined for each group $s$,
\begin{eqnarray*}
\upsilon _{1s,1} &\equiv &\frac{2}{n_{s}(n_{s}-1)}\sum_{i>j}H_{s,\{i,j\}}1\{%
\phi _{s,\{i,j\}}=1\}, \\
\upsilon _{2s,1} &\equiv &\frac{2}{n_{s}(n_{s}-1)}\sum_{i>j}1\{ \phi
_{s,\{i,j\}}=1\},
\end{eqnarray*}%
and defined $\upsilon _{1s,0}$, $\upsilon _{2s,0}$ analogously by replacing $%
\phi _{s,\{i,j\}}=1$ with $\phi _{s,\{i,j\}}=0$. Let $\upsilon _{s}\equiv
(\upsilon _{1s,1},\upsilon _{2s,1},\upsilon _{1s,0},\upsilon
_{2s.0})^{\prime }$.  We maintain the following regularity conditions:\medskip

\noindent (\textit{REG}) (i) $\exists \delta >0$ s.t. $\lim_{S\rightarrow \infty }\sum\nolimits_{s=1}^{S}E\left\{ \left\Vert Z_{s}^{\prime}R_{s}(p)\right\Vert ^{1+\delta }\right\} /(1+\delta )<\infty $; 
similar conditions hold for $Z_{s}^{\prime }Z_{s}$ and $Z_{s}^{\prime }\triangledown \left[ R_{s}(p)\theta \right] $. 
(ii) Let $\tau _{s}$, $\zeta _{s}$ be defined as in (\ref{AsyLP}) and (\ref{ASYM2}) below.
$\exists \delta ^{\prime }>0$ s.t. $E(||\tau _{s}||^{2+\delta ^{\prime }})<\infty $, and $S\times Var\left[S^{-1}\left( \sum_{s=1}^{S}\tau _{s}\right) \right] >0$ is bounded away from zero by some positive constants for $S$ large enough; similar conditions hold for $\zeta _{s}$.
\medskip

Under these conditions, we can apply appropriate versions of the law of large numbers, the central limit theorem, and the delta method to our sample which consists of observations $y_s, X_s, H_s$ that are independent and potentially heterogeneously distributed (due to the variation in group sizes $n_s$).

First, note our estimator for misclassification rates $\hat{p}$ is a
closed-form function of the sample averages of $\upsilon _{s}$. Thus the
asymptotic linear presentation of $\widehat{p}$ is 
\begin{equation} \label{AsyLP}
\sqrt{S}(\widehat{p}-p)=\tfrac{1}{\sqrt{S}}\sum\nolimits_{s}\underset{\equiv
\tau _{s}}{\underbrace{\mathcal{J}_{0}\times \left[ \upsilon _{s}-E(\upsilon
_{s})\right] }}+o_{p}(1)\text{,}
\end{equation}%
where $\mathcal{J}_{0}$ depends on the Jacobian matrix of $\hat{p}$ w.r.t.
the sample averages of $\upsilon _{s}$, evaluated at population counterparts. Next, note that by construction,%
\begin{eqnarray}
\sqrt{S}\left( \widehat{\theta }-\theta \right) &=&\sqrt{S}\left( \mathbf{A}%
^{\prime }\mathbf{B}^{-1}\mathbf{A}\right) ^{-1}\mathbf{A}^{\prime }\mathbf{B%
}^{-1}\mathbf{Z}^{\prime }\left[ Y-\mathbf{R}(\widehat{p})\theta \right] 
\notag \\
&=&\left( A_{0}^{\prime }B_{0}^{-1}A_{0}\right) ^{-1}A_{0}^{\prime
}B_{0}^{-1}\tfrac{1}{\sqrt{S}}\mathbf{Z}^{\prime }\left[ Y-\mathbf{R}(%
\widehat{p})\theta \right] +o_{p}(1)\text{,}  \label{ASYM1}
\end{eqnarray}%
where the second equality holds as $\mathbf{A}/S\overset{p}{\rightarrow 
}A_{0}$, $\mathbf{B}/S\overset{p}{\rightarrow }B_{0}$, $S^{-1/2}\mathbf{Z}%
^{\prime }\left[ Y-\mathbf{R}(\widehat{p})\theta \right] =O_{p}(1)$.

Recall the following definitions from the text:%
\begin{equation*}
F_{0}\equiv \lim_{S\rightarrow \infty
}S^{-1}\sum\nolimits_{s=1}^{S}E\left\{ Z_{s}^{\prime }\triangledown \left[
R_{s}(p)\theta \right] \right\} \text{.}
\end{equation*}%
For each group $s$ and individual $i\leq n_{s}$, let $R_{s,i}(p)$ denote the
corresponding row in $\mathbf{R}(p)$, and $\triangledown _{p}R_{s,i}(p)$ be
the $(K+1)$-by-$2$ Jacobian matrix of $R_{s,i}(p)$ with respect to $p$. Let $%
\triangledown _{p}\left[ R_{s}(p)\theta \right] $ denote an $n_{s}$-by-$2$
matrix with each row $i$ being $\theta ^{\prime }\triangledown _{p}R_{s,i}(p)
$, and let $\triangledown _{p}\left[ \mathbf{R}(p)\theta \right] $ be an $N$%
-by-$2$ matrix that stacks them for $s\leq S$. Then,%
\begin{eqnarray}
\tfrac{1}{\sqrt{S}}\mathbf{Z}^{\prime }\left[ Y-\mathbf{R}(\widehat{p}%
)\theta \right]  &=&\tfrac{1}{\sqrt{S}}\mathbf{Z}^{\prime }\left[ Y-\mathbf{R%
}(p)\theta \right] -\left( \tfrac{1}{S}\mathbf{Z}^{\prime }\triangledown _{p}%
\left[ \mathbf{R}(p)\theta \right] \right) \sqrt{S}(\widehat{p}-p)+o_{p}(1) 
\notag \\
&=&\tfrac{1}{\sqrt{S}}\sum\nolimits_{s}Z_{s}^{\prime }\left[
y_{s}-R_{s}(p)\theta \right] -F_{0}\left( \tfrac{1}{\sqrt{S}}%
\sum\nolimits_{s}\tau _{s}\right) +o_{p}(1)  \notag \\
&=&\tfrac{1}{\sqrt{S}}\sum\nolimits_{s}\underset{\equiv\zeta _{s}}{\underbrace{%
Z_{s}^{\prime }v_{s}-F_{0}\tau _{s}}}+o_{p}(1)\text{.}  \label{ASYM2}
\end{eqnarray}%
The first equality follows form a Taylor approximation around the actual
misclassification rates $p=(p_{0},p_{1})^{\prime }$; the second from $\tfrac{%
1}{S}\mathbf{Z}^{\prime }\triangledown _{p}\left[ \mathbf{R}(p)\theta \right]
\overset{p}{\longrightarrow }\lim_{S\rightarrow \infty
}S^{-1}\sum_{s}E\left\{ Z_{s}^{\prime }\triangledown _{p}\left[
R_{s}(p)\theta \right] \right\} $ and from the asymptotic linear
representation of the estimator $\widehat{p}=(\hat{p}_{0},\hat{p}_{1})$; the
third from $y_{s}=R_{s}(p)\theta +v_{s}$. This proves the limiting
distribution of $\sqrt{S}(\widehat{\theta }-\theta )$ in Proposition 5.

\section{A Single Large Network}\label{sub:singlenetwork}

In the main text, we focus on cases where the sample consists of many small, fixed-sized groups, where no links exist between members of different groups. For example, blocks could be villages or schools, with many links within each village or school, and practically no links between people in different villages or schools. 

We now show how an adjusted 2SLS also applies when there is interdependence between \textit{all} individuals in a sample. 
Specifically, we consider a setting in which the sample is partitioned into well-defined, \textit{approximate groups}, which we henceforth refer to as \textquotedblleft \textit{blocks}\textquotedblright. 
Formally, the individuals in the sample are partitioned into $S$ blocks. Links within each block $s$  are dense (i.e., the probability of forming links between individuals within the same block does \textit{not} diminish as the sample size increases);  
links between different blocks are sparse, with the rate of formation diminishing as the number of blocks increases. 

\subsection{A single large network setting}\label{sub: asinglenetwork}

The sample size is $N\equiv \sum_{s=1}^{S}n_{s}$. Let $G_{N}$ and $H_{N}$ denote the true and noisy measure of $N$-by-$N$ adjacency matrices respectively, which span the $S$ blocks in the sample.
Link misclassification exists in $H_N$ in two ways. 
First, links within each block are randomly misclassified in the sample at rates $p_0$ and $p_1$ as before. Second, the sparse cross-block links are \textit{never} reported in the sample, and so are missing.
Because all cross-block links are missing, $H_N$ is block-diagonal, with each diagonal block indexed as $H_{N,s}$ for $s=1,2,...,S$.

To facilitate derivation of the asymptotic properties of our 2SLS estimator, let $\widetilde{G}_{N}$ be a hypothetical \textit{block-diagonal approximation} of $G_{N}$, which perfectly reports all within-block links but drops all cross-block links. That is, for all individual $i$, 
\begin{equation*}
\widetilde{G}_{N,ij}=G_{N,ij}\text{ if }j\in s(i)\text{; }\widetilde{G}%
_{N,ij}=0\text{ if }j\notin s(i)\text{,}
\end{equation*}%
where $s(i)$ indicates the block that $i$ belongs to. 
By construction, all elements outside the diagonal blocks in $\widetilde G_N $ are zeros.
We maintain the following assumptions on the measurement errors in $H_{N}$:%
\begin{equation*}
\text{(N1) }E(H_{N,ij}|\widetilde{G}_{N},X)=E(H_{N,ij}|\widetilde{G}%
_{N,ij},X)\text{ }\forall i \neq j; %text{ and } j\in s(i).
\end{equation*}%
\begin{equation*}
\text{(N2) }E(H_{N,ij}|\widetilde{G}_{N,ij}=1,X)=1-p_1\text{, }E(H_{N,ij}|%
\widetilde{G}_{N,ij}=0,X)=p_0\text{ }\forall i \text{ and } j\neq i \text{ in } s(i).%\not=j\text{ and }p_0+p_1<1.
\end{equation*}%
As before, assume $p_0+p_1<1$. Furthermore, we maintain that the block-specific random arrays, $H_{N,s}$, $\widetilde{G}_{N,s}$, $X_{N,s}$, $\epsilon _{N,s}$ (with $H_{N,s},\widetilde{G}_{N,s}$ being $n_{s}$-by-$n_{s}$ matrices), are drawn independently across the blocks. 
Under these maintained conditions, we can consistently estimate the within block misclassification rates following the same approach as in Section 4. 
For the rest of this section, we take $(p_0,p_1)$ as given, and focus on the asymptotic properties of an adjusted 2SLS that removes misclassification bias by adjusting the diagonal block measures.

Let $W_N$ be a block-diagonal matrix, with each of its $S$ diagonal blocks adjusted as $W_{N,s} \equiv [H_{N,s}-p_0(\iota_{n_s}\iota'_{n_s}-I_{n_s})]/(1-p_0-p_1)$.
In the Web Appendix, we show that the structural model 
\[y_{N}=\lambda G_{N}y_{N}+X_{N}\beta +\varepsilon _{N}\]
% \begin{equation*}
%     % \label{eq:SF_nbd}
%     y_{N}=\lambda G_{N}y_{N}+X_{N}\beta +\varepsilon _{N}\text{,}
% \end{equation*}%  
can be written as
\begin{equation}
y_{N}=\lambda W_{N}y_{N}+X_{N}\beta +v_{N}+u_{N}\text{,}
\label{eq:noisy_SF_nbd}
\end{equation}%
% \begin{equation*}
where $u_{N}\equiv \left( I_{N}-\lambda W_N\right) \left(
I_{N}-\lambda \widetilde{G}_{N}\right) ^{-1}\lambda \Delta _{N}y_{N}$ 
with $\Delta _{N}\equiv G_{N}-\tilde{G}_{N}$ and
% \end{equation*}%
\begin{equation*}
v_{N}\equiv \varepsilon _{N}+\lambda \left( \widetilde{G}_{N}-W_N\right) \widetilde{y}_{N}\text{ with }\widetilde{y}_{N}\equiv
(I_{N}-\lambda \widetilde{G}_{N})^{-1}(X_{N}\beta +\varepsilon _{N})\text{.}
\end{equation*}
Note that we decompose composite errors in (\ref{eq:noisy_SF_nbd}) into $%
u_{N}$ and $v_{N}$, which are both vectorizations of block-specific vectors $u_{N,s}$ and $v_{N,s}$. 
While $v_{N,s}$ are independent across the blocks, $u_{N,s}$ are correlated across the blocks because of interdependence between $y_{N,s}$ due to sparse links between the blocks in $G_N$.
This difference requires us to apply separate tactics to characterize their contribution to the estimation errors.

This decomposition of the composite error is useful for illustrating two main steps for deriving the asymptotic result. 
Let $Z_N$ denote the matrix of instruments, with $Z_{N,s}$ being its sub-matrix specific to block $s$. Instrument exogeneity requires $E(Z_{N,s}'v_{N,s})=0$ for all $s$.
Recall the 2SLS estimator that uses $%
Z_{N}$ as instruments for $R_{N}\equiv
(W_{N}y_{N},X_{N})$ is $\widehat{\theta }=\left( A_{N}^{\prime }B_{N}^{-1}A_{N}\right)
^{-1}A_{N}^{\prime }B_{N}^{-1}Z_{N}^{\prime }y_{N}$, 
where $A_{N}\equiv Z_{N}^{\prime }R_{N}$ and $B_{N}\equiv Z_{N}^{\prime
}Z_{N}$. By definition,%
\begin{equation*}
\widehat{\theta }-\theta =\left( A_{N}^{\prime
}B_{N}^{-1}A_{N}\right) ^{-1}A_{N}^{\prime }B_{N}^{-1}Z_{N}^{\prime
}(v_{N}+u_{N})\text{.}
\end{equation*}%$
The asymptotic property of the estimator thus depends on that of $Z_{N}^{\prime }v_{N}$ and $Z_{N}^{\prime }u_{N}$, which we investigate sequentially.

First, we characterize the order of $Z_{N}^{\prime }v_{N}$, using the fact
that $v_{N,s}$ are independent across blocks $s$. 
To see why such independence holds, recall that $H_{N,s}$, $\widetilde{G}_{N,s}$, $X_{N,s}$, $\epsilon _{N,s}$ are assumed independent across blocks $s$. 
By construct, $\widetilde{G}_{N}$, $H_{N}$, $W_{N}$ and $(I-\lambda \widetilde{G}_{N})^{-1}$ are all block-diagonal. 
Hence $\widetilde{y}_{N,s}=(I_{s}-\lambda \widetilde{G}_{N,s})^{-1}(X_{N,s}\beta +\varepsilon _{N,s})$ are independent across $s$.%
\footnote{
    We refer to $\widetilde{y}_{N}$ as a \textit{hypothetical }reduced form, because it is based on the block-diagonal approximation $\widetilde{G}_{N}$ rather than the actual $G_{N}$.} 
It then follows that $v_{N,s}=\varepsilon
_{N,s}+\lambda \left( \widetilde{G}_{N,s}-W_{N,s}\right) 
\widetilde{y}_{N,s}$, and are independent across $s$.

We maintain exogeneity and independence conditions which are analogous to
(A3) and (A4) for the case with small groups in Section 3:%
\begin{eqnarray*}
\text{(N3)\ } &&E(\varepsilon _{N,s}|X_{N,s},G_{N,s},H_{N,s})=0\text{ for
all }s\text{;} \\
\text{(N4) } &&\text{Conditional on }(G_{N},X_{N})\text{, }H_{N,ij}\bot 
\text{ }H_{N,kl}\text{ for all }(i,j)\not=(k,l)\text{.}
\end{eqnarray*}%
Under these conditions, $E(v_{N,s}|X_{N,s},G_{N,s})=0$. 
The independence between $v_{N,s}$ mentioned above then allows us to apply the law of large numbers to show that 
\begin{equation*}
\frac{1}{S}Z_{N}^{\prime }v_{N}=\frac{1}{S}\sum
\nolimits_{s}Z_{N,s}^{\prime }v_{N,s}=O_{p}(S^{-1/2}).
\end{equation*}

Second, the order of $\frac{1}{S} Z_{N}^{\prime }u_{N}$ is bounded above by the expected number of misclassified links across the blocks, which are assumed to be sparse in the following sense:
\begin{equation*}
\text{(S-LOB)}\sum \nolimits_{i=1}^{N}\sum \nolimits_{j\not \in
s(i)}E\left( \left \vert \Delta _{N,ij}\right \vert \right) =O(S^{\rho })%
\text{ for some }\rho <1\text{.}
\end{equation*}%
This condition is the same as in \cite{lewbel2023ignoring}, who provide examples with primitive conditions. 
Among other things, it requires the links outside these blocks, or approximate groups, to be sparse with diminishing formation rates as $S\rightarrow\infty$.

\subsection{Asymptotic property of adjusted 2SLS in Section \ref{sub: asinglenetwork}}

We now derive the asymptotic property of adjusted 2SLS in the setting of a single, large network that is near-block diagonal, as defined in the previous subsection. 
Our objective is to show that, when the order of magnitude of the misclassification errors outside the diagonal blocks, or approximate groups, are small enough in the sense of (S-LOB), a 2SLS that only adjusts the link measure within each block while ignoring sparse, off-diagonal links is a root-n, consistent, asymptotically normal estimator for social effects.

Regularity conditions for deriving asymptotic properties are collected in Condition (S-REG). Suppose $I_{N}-\lambda G_{N}$ and $I_{N}-\lambda \widetilde{G}_{N}$ are invertible almost surely, and denote $M_{N}\equiv (I_{N}-\lambda G_{N})^{-1}$,  $\widetilde{M}_{N}\equiv (I_{N}-\lambda \widetilde{G}_{N})^{-1}$. Let $%
\widetilde{R}_{N,s}\equiv (W_{N,s}\widetilde{M}_{N,s}X_{N,s},X_{N,s})$.\medskip

\noindent (\textbf{S-REG}) (i) For all $i$, $\sup_{i}\left[ \sum
\nolimits_{j}|M_{N,ij}|\right] <\infty $; $\sup_{j}E\left( \left.
|X_{N,j}\beta |+|\varepsilon _{N,j}|\right \vert \Delta _{N}\right) <\infty $;

$\sup_{j}\left \vert \left( X_{N}^{\prime }H_{N}W_N\widetilde{M}_{N}\right)
_{ij}\right \vert <\infty $ and $\sup_{j}\left \vert \left( X_{N}^{\prime
}W_{N}\widetilde{M}_{N}\right) _{ij}\right \vert <\infty $ almost surely.

(ii) $(H_{N,s}$, $\widetilde{G}_{N,s}$, $X_{N,s}$, $\epsilon _{N,s})$ are
independent across blocks $s=1,2,...,S$.

(iii) There exist $\delta >0$ s.t. for all $s$, $E\left[ ||Z_{N,s}^{\prime }%
\widetilde{R}_{N,s}||^{1+\delta }\right] $, $E|\left[ ||Z_{N,s}^{\prime
}W_{N,s}\widetilde{M}_{N,s}\varepsilon _{N,s}||^{1+\delta }\right] $, and $%
E\left( \left \Vert Z_{N,s}^{\prime }Z_{N,s}\right \Vert ^{1+\delta }\right) 
$ are uniformly bounded.

(iv) For some $\delta >0$, $E\left \Vert Z_{N,s}^{\prime
}v_{N,s}\right
\Vert ^{2+\delta }<\Delta <\infty $ and $S^{-1}%
\sum_{s=1}^{S}Var(Z_{N,s}^{\prime }v_{N,s})>\delta ^{\prime }>0$ for $S$
sufficiently large.

(v) $\sup_{j}\left \vert \left[ \left( I_{N}-\lambda W_N%
\right) \widetilde{M}_{N}\right] _{ij}\right \vert <\infty $ for all $i$
almost surely.

(vi) $\lim_{S\rightarrow\infty }\frac{1}{S}\sum
\nolimits_{s}E\left( Z_{N,s}^{\prime }Z_{N,s}\right) $ and $%
\lim_{S\rightarrow\infty }\frac{1}{S}\sum \nolimits_{s}E\left(
Z_{N,s}^{\prime }\widetilde{R}_{N,s}\right) $ exist and are
non-singular.\medskip

Assumption (S-REG) collects regularity conditions needed for deriving the
asymptotic properties of $\widehat{\theta }-\theta$. Part (ii)
implies that exogenous variables are drawn independently across the blocks.
Part (i) and (v) introduce bound conditions on exogenous arrays in the
model. These allow us to relate differences between $y_{N}$ and its
near-block diagonal approximation $\widetilde{y}_{N}$ to the order of
difference between $G_{N}$ and $\widetilde{G}_{N}$. Parts (iii) and (iv) are
boundedness conditions on population moments that ensure a law of large
numbers and a central limit theorem apply to components of the
estimator.

Applying arguments similar to those in Proposition 3.1 and 3.2 of  \cite{lewbel2023ignoring}, we have the following proposition.

\begin{aproposition}
\label{pn:SLN_asymp} \textit{Suppose (N1), (N2), (N3) and (N4) hold. If
Assumptions (S-LOB) and (S-REG) hold, then}%
\begin{equation*}
\widehat{\theta }-\theta =O_{p}(S^{-1/2}\vee S^{\rho -1})\text{.}
\end{equation*}%
\textit{If in addition }$\rho <1/2$\textit{,} then%
\begin{equation*}
\sqrt{S}\left( \widehat{\theta }-\theta \right) \overset{d}{%
\longrightarrow }\mathcal{N}(0,\Omega )\text{,}
\end{equation*}
where $\Omega \equiv \left( A_{0}^{\prime }B_{0}^{-1}A_{0}\right)
^{-1}A_{0}^{\prime }B_{0}^{-1}\omega _{0}B_{0}^{-1}A_{0}\left( A_{0}^{\prime
}B_{0}^{-1}A_{0}\right) ^{-1}$ with $A_{0},B_{0},\omega _{0}$ being constant arrays defined in the appendix.
\end{aproposition}

To focus on this main goal, we take the misclassification rates $(p_0,p_1)$ as given and fixed in the adjustment.
(A proof that also accounts for estimation errors in the initial estimates of $(p_0,p_1)$ would follow from steps similar to Proposition 5 in Section 4.2, but do not add any insight for the main goal.) 
Also, for conciseness, we only investigate the case with a single, unsymmetrized measure as in Section 3.3.1; parallel results for the case of multiple, symmetrized measure follow from analogous arguments and are omitted for brevity.

We begin by deriving the noisy, feasible structural form in (17). % \ref{eq:noisy_SF_nbd}
First off, note that the reduced form of $y_{N}$ is:%
\begin{eqnarray}
y_{N} &=&(I_{N}-\lambda G_{N})^{-1}(X_{N}\beta +\varepsilon _{N})  \notag \\
&=&(I_{N}-\lambda \widetilde{G}_{N})^{-1}(X_{N}\beta +\varepsilon _{N})-%
\left[ (I_{N}-\lambda \widetilde{G}_{N})^{-1}-(I_{N}-\lambda G_{N})^{-1}%
\right] (X_{N}\beta +\varepsilon _{N})  \label{Redysingle} \\
&=&\underset{\equiv \widetilde{y}_{N}}{\underbrace{(I_{N}-\lambda \widetilde{%
G}_{N})^{-1}(X_{N}\beta +\varepsilon _{N})}}+(I_{N}-\lambda \widetilde{G}%
_{N})^{-1}\lambda \underset{\equiv \Delta _{N}}{\underbrace{(G_{N}-%
\widetilde{G}_{N})}}\underset{=y_{N}}{\underbrace{(I_{N}-\lambda
G_{N})^{-1}(X_{N}\beta +\varepsilon _{N})}}\text{.}  \notag %\label{Redysingle}
\end{eqnarray}%
where the third equality follows from the fact that $\mathcal{A}^{-1}-%
\mathcal{B}^{-1}=\mathcal{A}^{-1}(\mathcal{B}-\mathcal{A})\mathcal{B}^{-1}$
for invertible matrices $\mathcal{A}$, $\mathcal{B}$. Next, write (%\ref%{eq:SF_nbd}
14) as 
\begin{eqnarray*}
y_{N} &=&W_{N}y_{N}+X_{N}\beta +\varepsilon
_{N}+\lambda \left( \widetilde{G}_{N}-W_N\right)
y_{N}+\lambda \Delta _{N}y_{N} \\
&=&W_{N}y_{N}+X_{N}\beta +\underset{\equiv v_{N}}{%
\underbrace{\varepsilon _{N}+\lambda \left( \widetilde{G}_{N}-W_N\right) \widetilde{y}_{N}}+}\underset{\equiv u_{N}}{\underbrace{\lambda
^{2}\left( \widetilde{G}_{N}-W_N\right) (I_{N}-\lambda 
\widetilde{G}_{N})^{-1}\Delta _{N}y_{N}+\lambda \Delta _{N}y_{N}}}\text{,}
\end{eqnarray*}%
where the second equality holds because we substitute $y_{N}$ in $\lambda
\left( \widetilde{G}_{N}-W_N\right) y_{N}$ using the r.h.s.
of (\ref{Redysingle}). Furthermore, we can write 
\begin{equation*}
u_{N}=\left[ \lambda \left( \widetilde{G}_{N}-W_N\right)
(I_{N}-\lambda \widetilde{G}_{N})^{-1}+I_{N}\right] \lambda \Delta
_{N}y_{N}=\left( I_{N}-\lambda W_N\right) \left(
I_{N}-\lambda \widetilde{G}_{N}\right) ^{-1}\lambda \Delta _{N}y_{N}\text{.}
\end{equation*}%

\medskip

\noindent \textbf{Lemma A1.} \textit{Let }$a_{N}$\textit{, }$b_{N}$\textit{%
\ be random vectors in }$\mathbb{R}^{N}$.\textit{\ Suppose there exist
constants }$C_{1},C_{2}<\infty $\textit{\ such that }$\Pr \{ \sup_{i\leq
N}E(|a_{i}||\Delta _{N})\leq C_{1}\}=1$\textit{\ and }$\Pr \{ \sup_{j\leq
N}E\left( |b_{j}||\Delta _{N}\right) \leq C_{2}\}=1$\textit{.\ Then
Assumption S-LOB implies }$\frac{1}{S}a_{N}^{\prime }\Delta
_{N}b_{N}=O_{p}(S^{\rho -1})$.\medskip

\begin{proof}[Proof of Lemma A1]
From Assumption S-LOB, $\sum \nolimits_{i}\sum \nolimits_{j}E\left \vert
\Delta _{N,ij}\right \vert =O(S^{\rho })$\ for some $\rho <1$. By
construction,%
\begin{eqnarray*}
E\left( |\tfrac{1}{S}a_{N}^{\prime }\Delta b_{N}|\right) &\leq &\tfrac{1}{S}E%
\left[ \sup \nolimits_{i,j}E\left( |a_{i}b_{j}|\mid \Delta _{N}\right) \cdot
\left( \sum \nolimits_{i}\sum \nolimits_{j}|\Delta _{N,ij}|\right) \right]
\\
&\leq &\tfrac{1}{S}E\left[ C_{1}C_{2}\left( \sum \nolimits_{i}\sum
\nolimits_{j}|\Delta _{N,ij}|\right) \right] =O(S^{\rho -1})\text{.}
\end{eqnarray*}%
It then follows that $\tfrac{1}{S}a_{N}^{\prime }\Delta
_{N}b_{N}=O_{p}(S^{\rho -1})$.\ \ $\ \ $\medskip
\end{proof}

\noindent \textbf{Lemma A2. }\textit{Under the conditions in (S-REG)-(i),
there exists a constant }$C^{\ast }<\infty $\textit{\ such that }$\Pr \{
\sup_{i\leq N}E(|y_{i}||\Delta _{N})\leq C^{\ast }\}=1$\textit{\ for all }$N$%
.\medskip

\begin{proof}[Proof of Lemma A2]
Let $M_{N}\equiv (I_{N}-\lambda G_{N})^{-1}$. For any matrix $\mathcal{A}$,
let $\mathcal{A}_{(i)}$
%, $\mathcal{A}_{[k]}$ 
denote its $i$-th row; 
% and $k$ -th column respectively
and $\mathcal{A}_{ij}$ denote its $(i,j)$-th
component. It then follows from the reduced form that 
\begin{eqnarray*}
&&\sup_{i\leq N}E(|y_{N,i}|\mid \Delta _{N})=\sup_{i}E\left( \left. \left
\vert \sum \nolimits_{j}M_{N,ij}\left( X_{N,(j)}\beta +\varepsilon
_{j}\right) \right \vert \right \vert \Delta _{N}\right) \\
&\leq &\sup_{i}\left[ \sum \nolimits_{j}|M_{N,ij}|\right] \times
\sup_{j}E\left( \left. |X_{N,(j)}\beta |+|\varepsilon _{N,j}|\right \vert
\Delta _{N}\right) .
\end{eqnarray*}%
Hence, there exists some constant $C^{\ast }<\infty $ with $\Pr \{
\sup_{i}E(|y_{i}||\Delta _{N})\leq C^{\ast }\}=1$.\ \ $\ \ \medskip $
\end{proof}

\noindent \textbf{Lemma A3.} \textit{Under the conditions in (S-REG), }$%
\frac{1}{S}R_{N}^{\prime }Z_{N}=A_{0}+o_{p}(1)$\textit{, }$\frac{1}{S}%
Z_{N}^{\prime }Z_{N}=B_{0}+o_{p}(1)$\textit{, and }$\frac{1}{S}Z_{N}^{\prime
}v_{N}=O_{p}(S^{-1/2})$\textit{.}\medskip

\begin{proof}[Proof of Lemma A3]
By definition, $\frac{1}{S}Z_{N}^{\prime }Z_{N}=\frac{1}{S}\sum
\nolimits_{s=1}^{S}Z_{N,s}^{\prime }Z_{N,s}$, with $Z_{N,s}$ independent
across $s$ due to (S-REG)-(ii). Then by (S-REG)-(iii) and the law of large
numbers for independent and heterogeneously distributed observations (e.g.,
Corollary 3.9 in \cite{white2001asymptotic}), $\frac{1}{S}Z_{N}^{\prime
}Z_{N}=B_{0}+o_{p}(1)$ where $B_{0}\equiv \lim_{S\rightarrow \infty }%
\frac{1}{S}\sum \nolimits_{s}E\left( Z_{N,s}^{\prime }Z_{N,s}\right) $%
. Next, note by construction and (\ref{Redysingle}),%
\begin{equation}
\frac{1}{S}Z_{N}^{\prime }R_{N}=\frac{1}{S}\left( 
\begin{array}{cc}
X_{N}^{\prime }H_{N}W_N\widetilde{y}_{N} & X_{N}^{\prime }H_{N}X_{N} \\ 
X_{N}^{\prime }W_{N}\widetilde{y}_{N} & X_{N}^{\prime }X_{N}%
\end{array}%
\right) +\frac{1}{S}\lambda \left( 
\begin{array}{cc}
X_{N}^{\prime }{H}_{N}W_N\widetilde{M}_{N}\Delta _{N}y_{N} & 0 \\ 
X_{N}^{\prime }W_{N}\widetilde{M}_{N}\Delta _{N}y_{N} & 0%
\end{array}%
\right) \text{.}  \label{eq:C3_1}
\end{equation}%
By (S-REG)-(i) and Lemma A2, $y_{N}$ satisfies the condition on $b_{N}$ in
Lemma A1. It then follows from Lemma A1 that the \textit{second} term on the
right-hand side of (\ref{eq:C3_1}) is $O_{p}(S^{\rho -1})$. Besides, the 
\textit{first} term on the r.h.s. of (\ref{eq:C3_1}) is%
\begin{equation}
\frac{1}{S}\sum \nolimits_{s=1}^{S}Z_{N,s}^{\prime }\widetilde{R}_{N,s}+%
\frac{1}{S}\sum \nolimits_{s=1}^{S}\left( Z_{N,s}^{\prime }W_{N,s}%
\widetilde{M}_{N,s}\varepsilon _{N,s},\mathbf{0}\right) \text{.}
\label{eq:C3_2}
\end{equation}%
By (N3), $E\left( Z_{N,s}^{\prime }W_{N,s}\widetilde{M}_{N,s}\varepsilon
_{N,s}\right) =0$. It then follows from (S-REG)-(iii) that the expression in
(\ref{eq:C3_2})\ is $A_{0}+o_{p}(1)$, with $A_{0}\equiv
\lim_{S\rightarrow \infty }\frac{1}{S}\sum \nolimits_{s}E\left(Z_{N,s}^{\prime }\widetilde{R}_{N,s}\right) $.

Next, note that by definition,%
\begin{equation}
\frac{1}{S}Z_{N}^{\prime }v_{N}=\frac{1}{S}\sum
\nolimits_{s=1}^{S}Z_{N,s}^{\prime }\varepsilon _{N,s}+\lambda \frac{1}{S}%
\sum \nolimits_{s=1}^{S}Z_{N,s}^{\prime }\left( \widetilde{G}_{N,s}-W_{N,s}\right) \widetilde{y}_{N,s}\text{.}  \label{eq:C3_3}
\end{equation}%
By construction, $Z_{N,s}$, $\varepsilon _{N,s}$, $\widetilde{G}_{N,s}$ and $%
H_{N,s}$ are independent across blocks $s=1,2,...,S$. Also, recall that $%
\widetilde{y}_{N,s}$ is defined as $\widetilde{y}_{N,s}\equiv (I_{s}-\lambda 
\widetilde{G}_{N,s})^{-1}(X_{N,s}\beta +\varepsilon _{N,s})$, Hence $%
\widetilde{y}_{N,s}$ is also independent across the blocks. Assumption (N3)
implies $E(Z_{N,s}^{\prime }\varepsilon _{N,s})=0$; Assumptions (N1) and
(N2) imply 
\begin{equation*}
E\left( \left. W_{N,s}\right \vert \widetilde{G}_{N,s},X_{N,s}\right) =%
\widetilde{G}_{N,s}\text{.}
\end{equation*}%
Furthermore, the same argument as in the proof of Proposition 2 %\ref{pn:HX}
shows that under (N1), (N2), (N3) and (N4)%
\begin{equation*}
E\left( \left. H_{N,s}W_{N,s}\right \vert \widetilde{G}_{N,s},X_{N,s}\right)
=E\left( \left. H_{N,s}\widetilde{G}_{N,s}\right \vert \widetilde{G}%
_{N,s},X_{N,s}\right) \text{,}
\end{equation*}%
so that 
\begin{equation*}
E\left[ Z_{N,s}^{\prime }\left( \widetilde{G}_{N,s}-W_{N,s}%
\right) \widetilde{y}_{N,s}\right] =0\text{.}
\end{equation*}%
It then follows from (S-REG)-(iv) and the Central Limit Theorem that $\frac{1%
}{S}Z_{N}^{\prime }v_{N}=O_{p}(S^{-1/2})$. \ \ $\ $\medskip
\end{proof}

\begin{proof}[Proof of Proposition \ref{pn:SLN_asymp}]%\protect\ref{pn:SLN_asymp}
As shown in Lemma A3, $\frac{1}{S}R_{N}^{\prime }Z_{N}=A_{0}+o_{p}(1)$, $%
\frac{1}{S}Z_{N}^{\prime }Z_{N}=B_{0}+o_{p}(1)$, and $\frac{1}{S}%
Z_{N}^{\prime }v_{N}=O_{p}(S^{-1/2})$ under (N1)-(N4), (S-LOB) and (S-REG).
Furthermore, with (S-REG)-(v), Lemma A1 and Lemma A2 imply that $\frac{1}{S}%
Z_{N}^{\prime }u_{N}=O_{p}(S^{\rho -1})$. When $\rho <1/2$, we have
\begin{equation*}
\frac{1}{\sqrt{S}}Z_{N}^{\prime }(u_{N}+v_{N})\overset{d}{\rightarrow }\frac{%
1}{\sqrt{S}}Z_{N}^{\prime }v_{N}\overset{d}{\rightarrow }\mathcal{N}%
(0,\omega _{0}),
\end{equation*}%
where $\omega _{0}=\lim_{S\rightarrow \infty }\frac{1}{S}%
\sum \nolimits_{s}E\left( Z_{N,s}^{\prime }v_{N,s}v_{N,s}^{\prime
}Z_{N,s}\right) .${\small \ Hence,\ 
\begin{eqnarray*}
\sqrt{S}(\widehat{\theta }-\theta ) &=&\left( A_{0}^{\prime
}B_{0}^{-1}A_{0}\right) ^{-1}A_{0}^{\prime }B_{0}^{-1}\frac{1}{\sqrt{S}}%
Z_{N}^{\prime }v_{N}+{\small o_{p}(1)} \\
&&\overset{d}{\rightarrow }\mathcal{N}(0,\left( A_{0}^{\prime
}B_{0}^{-1}A_{0}\right) ^{-1}A_{0}^{\prime }B_{0}^{-1}\omega
_{0}B_{0}^{-1}A_{0}\left( A_{0}^{\prime }B_{0}^{-1}A_{0}\right) ^{-1}).
\end{eqnarray*}%
}

\end{proof}

\bibliographystyle{chicago}

\bibliography{missing_links}

\end{spacing}

\end{document}
